# Supplementary material for: VINet: Visual and Inertial-based Terrain Classification and Adaptive Navigation over Unknown Terrain
Source: arXiv:2209.07725 source file (2023-03-01)
Supplement: Supplementary file 1 [file trajectory_comp.tex]

\section{Trajectory Comparisons}
